# Supplementary material for: Room temperature, cavity-free capacitive strong coupling to mechanical motion
Source: arXiv:2407.15314 source file (2025-01-30)
Supplement: Supplementary file 1 [file supplement.pdf]

# Supplementary information for "Room temperature, cavity-free capacitive strong coupling to mechanical motion"

Denise Puglia,[1,*] Rachel Odessey,[1,2,†] Peter S. Burns,[1] Niklas Luhmann,[3] Silvan Schmid,[3] and Andrew P. Higginbotham[4,1,‡]

[1]*IST Austria, Am Campus 1, Klosterneuburg, 3400, Austria*
[2]*Pritzker School of Molecular Engineering, University of Chicago, 5640 S Ellis Ave, Chicago, IL 60637, United States*
[3]*Institute of Sensor and Actuator Systems, TU Wien, Gußhausstraße 27-29, Vienna, 1040, Austria*
[4]*James Franck Institute and Department of Physics, University of Chicago, 929 E 57th St, Chicago, Illinois 60637, USA*

## CONTENTS

I. Fundamental coupling considerations 3

II. Comparison with cavity optomechanics 3

III. Further experimental details 4
- A. Fabrication 4
- B. Measurement Setup 4
- C. Dimensions of the Setup 4
- D. Internal and External Coupling Extraction 4
- E. Butterworth-van Dyke model and circuit parameters fit 4
- F. Separation Distance Fit 5
- G. Inductor loss and $Q_L$ 5
- H. Frequency-dependent gain function G(f) 5
- I. Back-action noise from the measurement setup 5
- J. Dicke radiometer 5
- K. Expected mechanical temperature 6
- L. Sample parameters 6
- M. Voltage fluctuations in high impedance environment 6
- N. Higher Order Mechanical Modes 6

IV. Theoretical Model 8
- A. Continuum model 8
  - 1. Small dynamic displacement 8
  - 2. Static solution 9
  - 3. Effective 1D model 9
  - 4. Large dynamic displacements 10
- B. Collapse physics 10
- C. Dynamics 10
- D. Coupling to a circuit 10
  - 1. Antiresonance 11
  - 2. Mechanical damping from a transmission line 11
  - 3. Scattering parameters from Z 12
  - 4. Dissipation and resonant transmission 13
  - 5. Input-output theory 13
- E. Parametric gain 14
  - 1. Quadrature input-output theory 15
  - 2. Position inference 16

* Equal contribution; denise.puglia@ist.ac.at
† Equal contribution
‡ ahigginbotham@uchicago.edu

3. Signal recovery and apparent gain 17
F. Converting 2-port measurement into 1-port measurement 17
1. Conservation of energy in converted measurement 18
G. Added noise temperature 19
H. Cooperativity comparisons 19

## I. FUNDAMENTAL COUPLING CONSIDERATIONS

As discussed in the introduction, the impedance mismatch condition $Z_0/Z \ll 1$ is, for a linear geometry, equivalent to the Barginskiĭ and Manukin condition $v/c \ll 1$. To see why, note that the gate impedance in a linear geometry is approximately $Z \sim 1/(\omega\epsilon\lambda)$, where $\lambda$ is the mechanical wavelength. Using the relationship $\omega\lambda/(2\pi) = v_s$ leads to $Z_0/Z \sim v_s/c$, where we have approximated $Z_0$ by the impedance of free space, $Z_0 \sim \sqrt{\mu_0/\epsilon_0}$. In a two-dimensional parallel-plate geometry similar considerations yield $Z_0/Z \sim v_s\sqrt{A}/(cd)$, where $A$ is the plate area and $d$ is the plate separation. This is larger than the one dimensional case, but still small in practice. For instance, $v_s\sqrt{A}/(cd)$ would approach unity for macroscopic plates with $\sqrt{A} = 1$ m separated by 1 $\mu$m.

## II. COMPARISON WITH CAVITY OPTOMECHANICS

The physics of capacitive coupling between itinerant transmission-line modes and mechanical motion is discussed in the main text. It is illustrative to compare the behavior of this coupling with that of standard cavity optomechanical coupling. [6]. Both the cavity-free capacitive and cavity optomechanical couplings begin with a parametric interaction [Fig. S1], which modifies a parameter in the uncoupled Hamiltonian [56]. This parameter is the capacitance $C(x)$ in the case of cavity-free capacitive coupling and the resonant frequency $\omega(x)$ in the case of cavity optomechanical coupling.

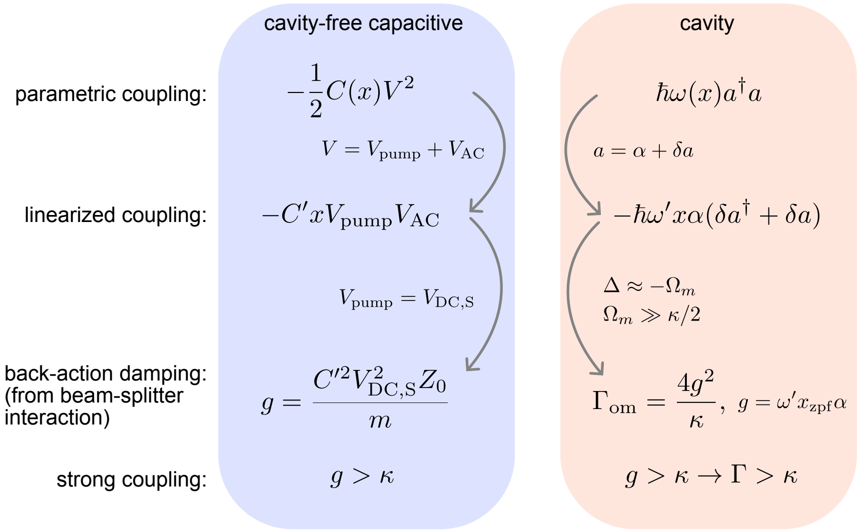


Figure S1. Comparison of cavity-free capacitive and cavity optomechanical couplings. Symbols in the left-hand column are the same as in the main text and the damping is for a single transmission-line device. Symbols in the right-hand column are from Ref. [6]: $\omega$ is the optical cavity frequency, $a$ is the photon lowering operator with classical pump strength $\alpha$ and quantum part $\delta a$, $b$ is the mechanical lowering operator, $g$ is the cavity-optomechanical coupling proportional to the zero-point position fluctuations $x_{\text{zpf}}$ and the pump strength $\alpha$, $\Delta$ is the pump-cavity detuning, and $\Gamma_{\text{om}}$ is the optomechanical back-action damping rate.

Cavity-free capacitive and cavity optomechanical parametric interactions can be linearized in the presence of a large pump. Both interactions generate back-action damping on mechanical motion under appropriate pumping: DC bias ($V_{\text{pump}} = V_{DC,S}$) for cavity-free capacitive or red-detuned $\Delta = -\Omega_m$ for cavity coupling. Both interactions, under the previously mentioned pumping conditions, can be viewed as beam-splitter type at the Hamiltonian level and have strong-coupling criteria that the coupling constant exceeds the cavity linewidth $g > \kappa$. In both cases these strong-coupling criteria imply that back-action damping exceeds cavity linewidth.

Note that $g$ in the cavity-free capacitive case is analogous to $\Gamma_{\text{om}}$ in the cavity optomechanics case. This is to some extent a choice of notation. However, it does reflect a real difference between the physical systems: there is only one rate in the cavity-free case, such that damping and coupling are identical.

## III. FURTHER EXPERIMENTAL DETAILS

### A. Fabrication

The experiment consists of two chips, a $Si_3N_4$ membrane and a bottom electrode, flipped on top of each other. The membrane was produced from Si wafers covered with 1.1 GPa stoichiometric $Si_3N_4$ on both sides. Using lithography, we define a window on the back of the wafer where $Si_3N_4$ was removed through reactive ion etch. Most of the $Si_3N_4$ on the front side of the wafer was also removed, leaving only a central square, which would become the 510-520 $\mu$m membrane, and smaller squares, which would become posts. The wafer was then dipped in KOH to etch the exposed silicon and release the membranes. We then evaporate 3 nm of Ti and 25 nm of Au on the released membranes. The electrode on the bottom chip was fabricated by evaporating 50 nm Pt on a high resistivity silicon wafer. We then evaporate 350 nm posts on the bottom chip, defining the separation distance between the bottom and top chip. The membrane chip was flipped on top of the electrode while carefully aligning the bottom and top posts. Finally, the two chips were glued with epoxy and bonded. The sample was loaded into a vacuum chamber and kept at around $10^{-5}$ mbar and room temperature. Figure 2 uses data from Sample 1, Figs. 3 and 4 use data from Sample 2, and Fig. 5 uses data from Sample 3.

### B. Measurement Setup

The measurements were conducted using a lock-in amplifier for the probe tone and, when present, an arbitrary waveform generator was used for the pump tone. For the two-port measurement, the pump and probe tones were added to the coupled port of a directional coupler. The mainline was grounded by a 50 ohm resistor. This AC signal was added to a DC bias through a bias-tee and connected to the back of the membrane. The transmitted radio wave would travel from the electrode directly to the input of the lock-in amplifier. The two-port measurement was converted to one-port with a 180 degrees hybrid coupler. The hybrid coupler recombines the scattering matrix elements with a phase, canceling the transmitted contributions and returning the reflection parameter $S_{11}$ at the output port. The incoming signal follows a similar path as for the two-port measurement, passing through the mainline of an extra directional coupler. Through the coupled port of this directional coupler, we can read out the reflected wave from the sample.

### C. Dimensions of the Setup

The data presented in this paper was acquired with a table-top setup occupying about 1 $m^2$. However, this space can be greatly reduced.A dedicated low loss inductor would require about 15x10x5 $mm^3$ of volume for a vacuum-sealed enclosure with an SMT connection for $V$. A rough estimate suggests that the parametric amplification with (or without) back-action isolation can be carried out in a 40x40x20 $mm^3$ enclosure with SMA connectors for $V$.

### D. Internal and External Coupling Extraction

In Fig. 2b, we extract $\kappa_{\text{in}}$ and $g$ from Lorentzian fits to the calibrated transmission data,

$$|S_{21}|^2 = \frac{g^2}{(2g+\kappa_{\text{in}})^2/4 + (\omega - \Omega_m)^2}. \tag{S1}$$

To be conservative, we include only cables leading up to the vacuum chamber in the calibration, leading to a slight underestimate of $g$ and an overestimate of $\kappa_{\text{in}}$.

### E. Butterworth-van Dyke model and circuit parameters fit

This circuit model includes a series RLC circuit ($R_{\text{eff}}$, $L_{\text{eff}}$, $C_{\text{eff}}$) in parallel with a gate capacitor ($C$). The gate capacitance is defined by the geometry of the metallized membrane at an equilibrium distance from the electrode. In terms of measurable and fitted variables it is determined by:

$$C = \frac{g}{Z_0(\Omega_a^2 - \Omega_m^2)}. \tag{S2}$$

Similarly, the series RLC circuit can be defined as:

$$C_{\text{eff}} = \frac{C^2 V_{\text{DC,S}}^2}{d^2} \frac{1}{m\Omega_m^2} \tag{S3}$$

$$L_{\text{eff}} = \frac{1}{\Omega_m^2 C_{\text{eff}}} \tag{S4}$$

$$R_{\text{eff}} = \kappa_{\text{in}} L_{\text{eff}}. \tag{S5}$$

To explain the shape of the antiresonance, an extra shunt resistor ($R_s$) is added in parallel to the Butterworth-van Dyke model. In Fig. 3a, we fit the transmission coefficient for the phase of the transmission coefficient as well as $C$, $\kappa_{\text{in}}$, $g$, $\Omega_m$, and $R_s$ (for CEM). The effective circuit parameters are then calculated as defined above.

### F. Separation Distance Fit

In Fig. 3b, we fit the squared resonance frequencies $\Omega_m^2$ to Eq. 2 with $d$ and $\Omega_0$ as fit parameters. The voltage shift is a fit of Eq. 1 to the voltage dependence of $g$. The membrane mass $m$ is calculated from the sample's design and optically-measured geometry. $C''(d, V_{\text{DC,S}})$ is calculated numerically accounting for the equilibrium deflection of the membrane due to $V_{\text{DC,S}}$ (see Supplement Eq. S20).

### G. Inductor loss and $Q_L$

In Fig. 3c, we present a metric for inductor quality factor or inductor loss calculated for the inductor region ($Im(Z) > 0$). The imaginary and real projections require a fit for the phase of the transmission coefficient. At the beginning of the inductive region, $Re(Z)$ and $Im(Z)$ are very small and the error of the phase fit can make $Q_L$ diverge. This can be observed in Fig. 3c in which a few data points present much larger $Q_L$ than the fit.

### H. Frequency-dependent gain function G(f)

The driven voltage fluctuations can be converted into undriven voltage fluctuations with the help of the frequency dependent gain function

$$G(f) = \frac{2\pi f - \frac{i\kappa}{2}}{2\pi f - i\kappa/(2G_A)}, \tag{S6}$$

where $G_A$ is the gain of the amplified quadrature, as discussed in the Supplement Section IV E.

### I. Back-action noise from the measurement setup

The back-action noise from our measurement setup was determined by attaching several different external resistors to the apparatus input while measuring voltage noise at the output. We found an input voltage noise of 4 nV/$\sqrt{\text{Hz}}$, matching the manufacturer's specification for our instrument, and an input current noise of 25 pA/$\sqrt{\text{Hz}}$. In the un-isolated setup, we estimate that this current noise will heat mechanical motion to a temperature of approximately 484 K, close to the excess thermomechanical noise measured in Fig. 4.

### J. Dicke radiometer

The error bars presented in Fig. 5c are given by the sensitivity of the Dicke radiometer, a common metric for thermally-emitted electromagnetic radiation. For an ideal Dicke radiometer, the standard deviation of the area ($\sigma_A$) is:

$$\sigma_A = \sqrt{\frac{A_a}{N_a/2} + \frac{A_w}{N_w/2}}, \tag{S7}$$

where $A_{a/w}$ is the area contribution from the amplified thermomechanical fluctuations/white noise, and $N_{a/w}$ is the number of independent samples contributed by the same sources. The white noise is uncorrelated, so $N_w$ is simply the length of the trace divided by the sampling time ($t_s$). However, the amplified thermomechanical fluctuations are correlated and $N_a$ must correct the independent number of points, dividing it by $N_{\text{corr}}$:

$$N_{\text{corr}} = \frac{2}{\kappa/G_A t_s}, \tag{S8}$$

where $\kappa/G_A$ is the bandwidth.

### K. Expected mechanical temperature

In Fig. 5c, the expected mechanical temperature $T_m$ is 295 K for the room temperature load because all system components are in thermal equilibrium. For the cold load, the expected mechanical temperature is given by $T_m = (2g/\kappa)T_{\text{in}} + (\kappa_{\text{in}}/\kappa)T_{\text{RT}}$ where $T_{\text{RT}} = 295$ K and $T_{\text{in}}$ is the input radiation temperature. The parameters $g$, $\kappa_{\text{in}}$, and $\kappa$ are fixed from measured scattering parameters and $T_{\text{in}} = 105$ K from the temperature of liquid nitrogen and the measured insertion loss from the cold load to the sample.

### L. Sample parameters

Three samples were measured to produce the data for the paper. The geometric parameters of the samples are as follows:

| parameter | Sample 1 | Sample 2 | Sample 3 |
|---|---|---|---|
| $L$ ($\mu$m) | 514 | 520 | 511 |
| $d$ (nm) | 226 | 321 | 607 |
| $m$ (ng) | 185 | 189 | 182 |
| $t_{\text{metal}}$ (nm) | 28 | 28 | 28 |
| $\Omega_0/2\pi$ (kHz) | 500 | 380 | 389 |
| $\kappa_{\text{in}}$ (Hz) | 36±8 | 5±2 | 9±6 |

Table SI. Geometric and resonance parameters of the three samples used in the paper. For geometric parameters, $L$ is the membrane side length, $d$ is the separation distance of the top and bottom chip, $m$ is the membrane mass, and $t_{\text{metal}}$ is the deposited metal thickness. For resonance parameters, $\Omega_0/2\pi$ is the resonant frequency and $\kappa_{\text{in}}$ is the internal dissipation calculated at zero effective voltage.

### M. Voltage fluctuations in high impedance environment

This section presents data to support the claim that gain fluctuations do not impair the functionality of the parametric amplifier in a high impedance environment. Figure S2 shows raw demodulated X- and Y-quadratures for the setup introduced in Fig.4 of the main text, but in a high impedance environment. The equivalent gain of 5 remains constant for a period of about 5 minutes and no instabilities are observed.

### N. Higher Order Mechanical Modes

This section presents data from higher order mechanical modes acquired at fixed DC voltage and with the measuring circuit already used in Fig. 2a of the main text. An increase in the insertion loss can be observed for higher frequency modes. Note that this data is from a fourth sample not included in [Table SI].

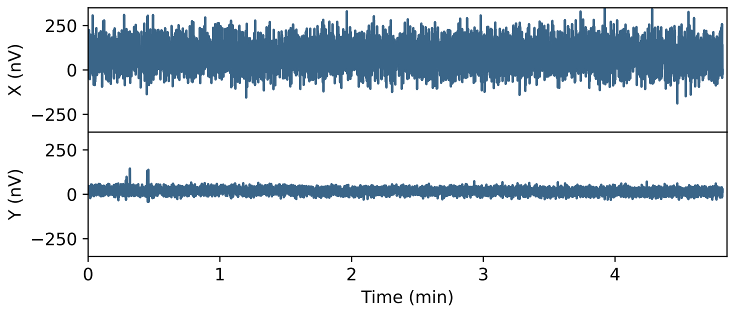


Figure S2. Voltage fluctuations in a high impedance environment taken using the setup introduced by Fig.4 of the main text.

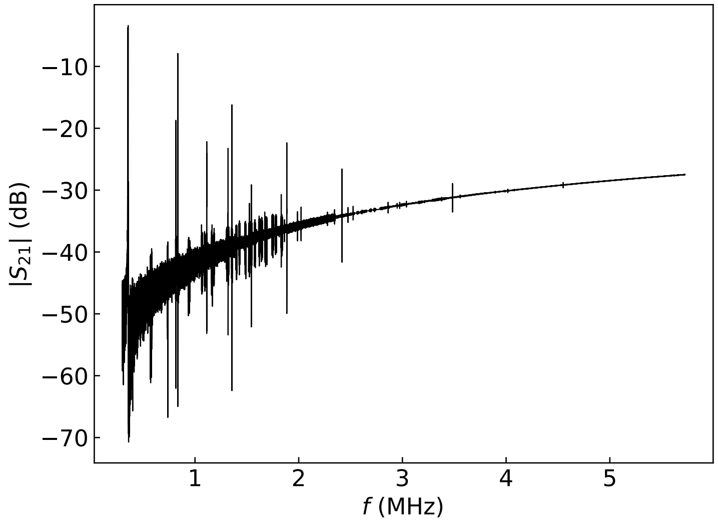


Figure S3. $S_{21}$ transmission parameter at fixed DC bias voltages as a function of frequency.

## IV. THEORETICAL MODEL

A simple way to understand thee experiment is to view it as a 1D problem of a mechanically compliant capacitor as shown in Fig. 1 of the main paper. It consists of a metallized silicon nitride membrane suspended over a stationary electrode with plate separation $d$. The 2D membrane maps on to this problem with some effective mass $m$, mechanical spring constant $k_0$, and capacitance $C$, which we cover later in Sec. IV A. For the 1D problem, we consider a mechanical spring coupled to an electrical spring $H_{\text{int}} = -\frac{1}{2}C(x)V_{\text{DC}}^2$ where capacitance depends on the deflection of the spring and $V_{\text{DC}}$ is applied DC bias. For the theoretical model, we consider that the applied $V_{\text{DC}}$ is directly felt by the sample without the presence of a voltage shift ($V_{\text{DC}} = V_{\text{DC,S}}$) . If we consider $x$ to be the 1D coordinate of deflection of the mechanical spring from its equilibrium position in the absence of an applied DC bias, we can write a Hamiltonian for the system:

$$H = \frac{p^2}{2m} + \frac{1}{2}k_0x^2 + H_{\text{int}}, \tag{S9}$$

where $p$ represents the momentum. From here forward, unless otherwise specified, we assume that $C$ and its spatial derivatives $C'$ and $C''$ are evaluated when $x$ is at its mechanical equilibrium value $x = x_{\text{eqm}}$. Expanding the capacitance about equilibrium gives

$$H_{\text{int}} = -\frac{1}{2}C(x)V^2 \approx -\frac{1}{2}CV^2 - \frac{1}{2}C'V^2x - \frac{1}{4}C''V^2x^2. \tag{S10}$$

The last term gives rise to an electrostatic spring constant, $k_e = -\frac{1}{2}C''V^2$, which is responsible for parametric electromechanical coupling. The second term indicates the presence of an electrostatic force, $1/2C'V^2$, which couples the mechanical resonator to propagating voltages. Considering a transmission line of impedance $Z_i$, the mechanical oscillator couples to the propagating voltages at a rate $g_i = C'^2V_{\text{DC}}^2Z_i/m$ and to a dissipative bath at a rate $\kappa_{\text{in}}$. The total mechanical linewidth is $\kappa_{\text{in}} + g_1 + g_2 + ...$ . Considering a standard line impedance of 50 Ω ($Z_0$) and $V_{\text{DC}}$ below 30 V to facilitate integration to other circuit elements, it is necessary to carefully choose the geometry parameters to reach the strong coupling limit $g_i > \kappa_{\text{in}}$.

### A. Continuum model

We start our endeavor by imagining a rectangular membrane with side lengths $L_y, L_z$ and 2D density $\rho_{2\text{D}}$, under a pre-stress $\sigma$. It is described by a continuum Lagrangian density [57]

$$\mathcal{L} = \mathcal{T} - \mathcal{V} = \frac{1}{2}\rho_{2\text{D}}\dot{u}^2 - \frac{1}{2}\sigma h|\nabla u|^2 - \mathcal{U}, \tag{S11}$$

where $h$ is the thickness of the membrane, $\mathcal{U} = -\frac{1}{2}\frac{\epsilon_0}{d+u}V^2$ is the electromechanical interaction energy, and $u(V, y, z, t)$ is the 2D continuum displacement from the zero-bias equilibrium position in the vertical direction, with $\epsilon_0$ being the vacuum permittivity and $V$ the total voltage.

#### 1. *Small dynamic displacement*

We will allow for large static displacements plus a small dynamic part. Assuming that the dynamic part does not effect the static solution, justified only for small dynamics, we will independently solve the static problem and expand about this solution to find the dynamics. The static problem is solved in Sec. IV A 2.

To expand around the static solution, we separate variables into static and dynamic parts $V(t) = V_{\text{DC}} + V_{\text{AC}}$, and $u(V, y, z, t) = u_0(V_{\text{DC}}, y, z) + u_1(V_{\text{AC}}, y, z, t)$. Expanding $\mathcal{U}$ up to quadratic order in dynamical variables and neglecting terms that couple $u_0$ and $V_{\text{AC}}$ gives

$$\mathcal{U} \approx -\frac{\epsilon_0}{2(d+u_0)}V_{\text{DC}}^2 + \frac{\epsilon_0}{2(d+u_0)^2}u_1(V_{\text{DC}}^2 + 2V_{\text{DC}}V_{\text{AC}}) - \frac{\epsilon_0}{2(d+u_0)^3}u_1^2V_{\text{DC}}^2. \tag{S12}$$

Inserting this expansion into Eq. S11, the Lagrangian density breaks into static and dynamic parts $\mathcal{L} = \mathcal{L}_0 + \mathcal{L}_1(t)$. The static Lagrangian density $\mathcal{L}_0$ is identical to Eq. S14, which gives the static displacement. The dynamic Lagrangian density is

$$\mathcal{L}_1 = \frac{1}{2}\rho_{2\text{D}}\dot{u_1}^2 - \frac{1}{2}\sigma h|\nabla u_1|^2 + \frac{\epsilon_0}{2(d+u_0)^3}u_1^2V_{\text{DC}}^2 - \frac{\epsilon_0}{(d+u_0)^2}u_1V_{\text{DC}}V_{\text{AC}}. \tag{S13}$$

To arrive at the expression for the static Lagrangian density, we cancel the cross term $\sigma h \nabla u_0 \cdot \nabla u_1$ arising from the expansion of the mechanical potential with the static $u_1 V_{\mathrm{DC}}^2$ in Eq. S12 by making use of the equations of motion for $u_0$ (Eq. S15) and the boundary conditions of $u_1$. Physically, this is a consequence of the fact that static forces must balance in equilibrium.

### *2. Static solution*

Starting from Eq. S11, we seek a static solution $u_0$ with $\dot{u_0}$=0. $u_0$ has the Lagrangian density $\mathcal{L}_0$

$$\mathcal{L}_0 = -\frac{1}{2}\sigma h |\nabla u_0|^2 + \frac{1}{2}\frac{\epsilon_0 V_{\mathrm{DC}}^2}{d+u_0}. \tag{S14}$$

The Euler-Lagrange equation gives the equilibrium condition for $u_0$,

$$\sigma h \nabla^2 u_0 = \frac{\epsilon_0 V_{\mathrm{DC}}^2}{2(d+u_0)^2}. \tag{S15}$$

Expanding the above expression for $u_0 \ll d$ results in a linear equation of motion, which is solved in terms of the Fourier series $u_0(V,y,z) = \sum_{a,b} \ell_{ab}(V) f_{ab}(y,z)$ with $f_{ab}(y,z) = \sin(\frac{a\pi y}{L_y})\sin(\frac{b\pi z}{L_z})$. The Fourier coefficients $\ell_{ab}$ are

$$\ell_{ab}(V) = -\frac{8\epsilon_0 V_{\mathrm{DC}}^2 \Phi_{ab}/(d^2\pi^2 ab)}{\rho_{2D}\Omega_{0,ab}^2 - \frac{\epsilon_0 V_{\mathrm{DC}}^2}{d^3}}, \tag{S16}$$

where $\Omega_{0,ab}$ is the zero voltage mechanical frequency for modes $a$, $b$, and $\Phi_{a,b}$ is the mode matching factor with $\Phi_{a,b} = \frac{ab\pi^2}{4L_yL_z}\iint_{\mathcal{S}} \sin(\frac{a\pi y}{L_y})\sin(\frac{b\pi z}{L_z})dydz$, where $\mathcal{S}$ is the electrode surface under the membrane. In case of perfect electrode-membrane overlap, $\Phi_{a,b} = 1$ for $a$, $b$ odd and $\Phi_{a,b} = 0$ if $a$ or $b$ is even. The expression above reduces to $\ell_{ab} = \frac{2C'_{pp}V_{\mathrm{DC}}^2\Phi_{a,b}}{\pi^2 abm\Omega_{pp,ab}^2}$, with $\Omega_{pp,ab}^2 = \Omega_{0,ab}^2 - \Omega_{e,pp}^2$, $C'_{pp} = -\epsilon_0 L_y L_z/d^2$ and an electromechanical frequency shift in the parallel capacitor approximation $\Omega_{e,pp}^2 = \frac{\epsilon_0 V_{\mathrm{DC}}^2 L_y L_z}{4md^3}$.

### *3. Effective 1D model*

To create an effective model, one may decompose the displacement into a sum of normal modes times an amplitude function $x_{n,j}(t)$,

$$u_{1,nj}(y,z,t) = x_{n,j}(t)\sin\left(\frac{n\pi y}{L_y}\right)\sin\left(\frac{j\pi z}{L_z}\right) \tag{S17}$$

and insert into the linearized Lagrangian density. Due to the orthogonality of the normal modes, the Lagrangian $L_1 = \int dydz\mathcal{L}_1$ becomes a sum of independent contributions from each normal mode, $L_1 = \sum_{n,j} L_{1,n,j}$. Each normal mode is equivalent to a simple harmonic oscillator with position $x_{\mathrm{n,j}}$,

$$L_{1,n,j} = \frac{1}{2}m\dot{x}_{n,j}^2 - \frac{1}{2}m\Omega_{m,nj}^2 x_{n,j}^2 + C' V_{\mathrm{DC}} V_{\mathrm{AC}} x_{n,j}. \tag{S18}$$

The effective mass is $m = \rho_{\mathrm{2D}} L_x L_y/4$. The resonance frequency is given by

$$\Omega_{m,nj}^2 = \Omega_{0,nj}^2 - \Omega_e^2 \tag{S19}$$

where $\Omega_{0,nj}^2 = \frac{\sigma h}{\rho_{\mathrm{2D}}}\left(\frac{\pi^2 n^2}{L_y^2} + \frac{\pi^2 j^2}{L_z^2}\right)$ is the bare resonant frequency and $\Omega_e^2 = C'' V_{\mathrm{DC}}^2/2m$ is the electromechanical frequency shift. The capacitance $C = \int \frac{\epsilon_0}{d+u_0} dydz$ and its derivatives

$$C' = -\int \frac{\epsilon_0 \sin\left(\frac{n\pi y}{L_y}\right)\sin\left(\frac{j\pi z}{L_z}\right)}{(d+u_0)^2}dydz, C'' = 2\int \frac{\epsilon_0 \sin^2\left(\frac{n\pi y}{L_y}\right)\sin^2\left(\frac{j\pi z}{L_z}\right)}{(d+u_0)^3}dydz \tag{S20}$$

can be calculated numerically. Equation S18 defines a 1D model equivalent to the electromechanical spring model introduced in Eq. S9.

### *4. Large dynamic displacements*

We derived an effective 1D model under the assumption of small dynamic displacements. This assumption can be relaxed by instead taking advantage of the fact that we have a high-$Q$ system and making use of a rotating wave approximation. Instead of expanding the Lagrangian in orders of $V_{\mathrm{AC}}$, $u_1$ and neglecting coupling between $u_0$ and $V_{\mathrm{AC}}$, we can instead collect terms in the Lagrangian oscillating at $0\omega$, $\omega$, $2\omega$. The upshot is that there is now a static contribution from $\langle V_{\mathrm{AC}}^2 \rangle$, where $\langle . \rangle$ denotes a time average. One can include this term by using the formulae in Sec. IV A 3 with the substitution

$$V_{\mathrm{DC}}^2 \to V_{\mathrm{DC}}^2 + \langle V_{\mathrm{AC}}^2 \rangle. \tag{S21}$$

## B. Collapse physics

As shown in Eq. S19, the DC voltage causes corrections to the mechanical resonant frequency $\Omega_m$ according to $\Omega_m^2 = \Omega_0^2 - \Omega_e^2$. The equilibrium position $x_{\mathrm{eq}}$ also depends on voltage. The dependence can found exactly by minimizing the potential part of the energy, solving

$$x_{\mathrm{eq}} = \frac{C'(x_{\mathrm{eq}})V^2}{2m\Omega_m^2}. \tag{S22}$$

Since $C'$ depends on $x$, this gives a cumbersome expression. The important result is that for sufficiently strong voltages there are no longer stable minima. A parallel-plate capacitor with plate separation $d$ then collapses once $x_{\mathrm{eq}}/d \approx 0.67$.

## C. Dynamics

We return to the dynamic Lagrange equations (Eq. S18) for a single mode,

$$m\ddot{x} = -m\Omega_m^2 x + C' V_{\mathrm{DC}} V_{\mathrm{AC}}, \tag{S23}$$

where we have have dropped the $n, j$ subscripts for convenience. We want to consider an applied voltage $V_{\mathrm{AC}} = |V_{\mathrm{AC}}| \cos \omega t$ and add a phenomenological damping parameter $\kappa_{\mathrm{in}}$ to describe mechanical dissipation. With these changes, we obtain the linearized equation of motion

$$m\ddot{x} = -m\Omega_m^2 x - m\kappa_{\mathrm{in}}\dot{x} + F_{\mathrm{em}}, \tag{S24}$$

where $F_{\mathrm{em}} = C' V_{\mathrm{DC}} |V_{\mathrm{AC}}| \cos \omega t$ is the electrostatic force. We can also write (S24) in the frequency domain as follows:

$$-\omega^2 x = -\Omega_m^2 x - i\omega\kappa_{\mathrm{in}} x + F_{\mathrm{em}}/m, \tag{S25}$$

where we have divided by $m$ for simplicity. This equation is solved in frequency space by

$$x = \chi_m F_{\mathrm{em}}/m, \tag{S26}$$

where $\chi_m = (\Omega_m^2 - \omega^2 + i\kappa_{\mathrm{in}}\omega)^{-1}$ is the mechanical susceptibility and $i$ is the imaginary unit. Note that since C' considers the mode matching factor, the force will be zero for even modes coupled to an electrode with full overlap. Note also that if $V_{\mathrm{AC}} = |V_{\mathrm{AC}}| cos(\omega_2 t)$ and $\omega_2 >> \omega$, than the force component at $\omega$ is zero and therefore $x(\omega)$ is zero.

## D. Coupling to a circuit

To understand coupling to an electrical circuit, one may start with the constitutive relation for a capacitor $q = CV$. Differentiating gives $I = \dot{C}V + C\dot{V}$. Given a varying current $I = I_0 + I_1 e^{i\omega t}$, we again keep only terms oscillating at $\omega$, arriving at

$$I_1 = i\omega C' x V_{\mathrm{DC}} + i\omega C V_{\mathrm{AC}}. \tag{S27}$$

Finally, inserting the solution for $x$ gives

$$I_1 = (Z_m^{-1} + Z_C^{-1})V_{\rm AC}, \tag{S28}$$

where the mechanical impedance is $Z_m^{-1} = i\omega C'^2 V_{\rm DC}^2 \chi_m/m$. As pointed out in Ref. [25], one can now construct an effective circuit model consisting of the mechanical impedance in parallel with the capacitor impedance $Z_C^{-1} = i\omega C$. The membrane impedance is equivalent to that of a series RLC circuit with parameters

$$C_{\rm eff} = \frac{C'^2 V_{\rm DC}^2}{m\Omega_m^2} \tag{S29}$$

$$L_{\rm eff} = \frac{1}{\Omega_m^2 C_{\rm eff}} \tag{S30}$$

$$R_{\rm eff} = \kappa_{\rm in} L_{\rm eff}. \tag{S31}$$

This gives the expected circuit resonant frequency of $\Omega_m$ and linewidth $\kappa_{\rm in}$. A key insight is that for typical silicon nitride membranes and moderate voltages, one can already obtain $R \sim 50\ \Omega$. Thus, the odd modes of the mechanical oscillator can be matched to the transmission line.

### 1. *Antiresonance*

The balancing of a gate capacitance by the RLC circuit gives rise to an antiresonance. The antiresonance occurs when the imaginary part of the total reactance $Y$ is zero. Using $Y = Y_m + Y_C$ and $Y_m = i\omega g \chi_m/Z_0$ gives an approximate expression for the antiresonance frequency $\Omega_a$

$$\Omega_a^2 = \Omega_m^2 + \frac{g}{Z_0 C}, \tag{S32}$$

valid when the antiresonance is detuned from $\Omega_m$ by much more than a linewidth. When the linewidth is dominated by coupling, this condition is equivalent to $1/(\Omega_m C) \gg Z_0$, which is well satisfied even for the largest achievable capacitances.

For analysis of the antiresonance frequency, it is useful to express $\Omega_a$ in terms of the bare mechanical resonance and geometric quantities. Combining with the bias-dependence of resonance frequency (see Sec. IV A 2) gives

$$\Omega_a^2 = \Omega_0^2 + \left(\frac{C'^2}{C} - \frac{C''}{2}\right)\frac{V_{\rm DC}^2}{m}, \tag{S33}$$

where $C$, $C'$, and $C''$ are determined numerically (Eq. S20).

### 2. *Mechanical damping from a transmission line*

A physical view of damping can be given by writing down a dressed mechanical susceptibility due to the electromechanical interaction. To do this, let's think about a minimal setup where the oscillator is coupled to a single port through a transmission line with impedance $Z_0$. An incoming wave generates a force proportional to $V_{\rm AC}^+$. However, Eq. S24 considers an external driving force proportional to $V_{\rm AC} = V_{\rm AC}^+ + V_{\rm AC}^-$. This reflects the fact that a reflected wave will be generated by the mechanical oscillator, which also generates a force. As we will see below, the force from this reflected wave is responsible for damping.

To see how this comes about, we need to write the mechanical susceptibility to the applied force, which is proportional to $V_{\rm AC}^+$. Differentiating $q = CV$ and inserting the expression for current $I = (V_{\rm AC}^+ - V_{\rm AC}^-)/Z_0 = (2V_{\rm AC}^+ - V_{\rm AC})/Z_0$ we find the expression

$$V = 2V_{\rm AC}^+ - i\omega C' Z_0 x V_{\rm DC}, \tag{S34}$$

where we have neglected the effect of the gate capacitance for simplicity.

Inserting this result into the frequency-domain version of Eq. S24 we find

$$-\omega^2 x = -\Omega_m^2 x - i\omega\left(\kappa_{\rm in} + \frac{Z_0 (C' V_{\rm DC})^2}{m}\right)x + 2C' V_{\rm DC} V_{\rm AC}^+/m. \tag{S35}$$

We can immediately see that the susceptibility to an incident wave $\overline{\chi}_m = (\Omega_m^2 - \omega^2 + i\kappa_{\text{eff}}\omega)^{-1}$ is dressed with an effective damping rate

$$\kappa_{\text{eff}} = \kappa_{\text{in}} + g, \tag{S36}$$

where $g = \frac{Z_0(C'V_{\text{DC}})^2}{m}$ is the electromechanical coupling. We can then write the mechanical displacement on the incoming signal,

$$x = 2\sqrt{\frac{g}{m}}\overline{\chi}_m \frac{V_{\text{AC}}^+}{\sqrt{Z_0}}. \tag{S37}$$

*3. Scattering parameters from Z*

Now that we have a model for the impedance seen by the transmission line, $Z^{-1} = Z_m^{-1} + Z_C^{-1}$, scattering parameters can be written down for the three possible configurations of the transmission line: with a single port, with two identical ports, and with two different ports. To treat different line impedances symmetrically, its useful to work with power waves, defined for instance by

$$v_1^+ = V_1^+/\sqrt{Z_0}, \tag{S38}$$

where $V_{\text{i}}^+$ is the incident wave on port $i$. Note that $|v_1^+(t)|^2$ then has units of power and $|v_1^+(f)|^2$ has units of energy spectral density. This also makes them nice to work with from the perspective of thermodynamics.

*a. 1 port*

In a one-port reflection configuration one has $S_{11} = (Z - Z_0)/(Z + Z_0)$ where $Z_0$ is the characteristic impedance of the transmission line. A simple limit for understanding the results is to work near resonance and neglect the gate impedance, taking $Z \approx Z_m$. One then finds

$$S_{11} \approx 1 - \frac{2Z_0}{Z_0 + Z_m} \tag{S39}$$

$$= 1 - 2ig\omega\overline{\chi}_m. \tag{S40}$$

The same expression can also be found by neglecting gate capacitance in Eq. S27, which gives $v^- = v^+ - i\omega\sqrt{gm}x$, and then combining with Eq. S37.

What is the temperature of the mechanical oscillator? In the limit that the dominant coupling is to the transmission line ($g$ large) the position spectral density $S_{\text{xx}}$ is related to the electrical power spectral density of $v_1^+$, $S_{+,+}$ by

$$S_{\text{xx}} = 4\frac{g}{m}|\overline{\chi}_m|^2 S_{+,+}. \tag{S41}$$

Using $\int_0^\infty |\overline{\chi}_m|^2 = 1/(\kappa\Omega_m^2)$, and equipartition $k_B T_m = m\Omega_m^2\langle x^2\rangle$ we find, $k_B T_m = S_{+,+}$, where $k_B$ is the Boltzmann constant. If port 1 is in equilibrium then Johnson-Nyquist noise gives $S_{+,+} = k_B T_+$, so

$$T_m = T_+, \tag{S42}$$

confirming that the mechanics equilibrates with the transmission line when it is strongly coupled.

*b. 2 port*

In a 2-port transmission configuration $S_{21} = 2Z_0/(2Z_0 + Z)$. For general transmission-line impedances on ports one ($Z_1$) and two ($Z_2$), the transmission is $2Z_2/(Z_1 + Z_2 + Z) \cdot \sqrt{Z_1/Z_2}$, where the last factor is present because we work with power waves. One can see that when $R_{eff} \ll Z_2$ one approaches unity transmission on resonance. Thus, the mechanical oscillator acts as a low-insertion loss bandpass filter. The reflection coefficient from port 1 is $S_{11} = 1 - 2Z_1/(Z_1 + Z_2 + Z)$.

One can then proceed in analogy with Sec. IV D 3 a to find scattering parameters. For instance, one finds

$$S_{21} = 2i\omega\sqrt{g_1 g_2}\overline{\chi}_m \tag{S43}$$

$$S_{11} = 1 - 2i\omega g_1\overline{\chi}_m. \tag{S44}$$

where now

$$\kappa_{\text{eff}} = \kappa_{\text{in}} + g_1 + g_2, \tag{S45}$$

and the coupling constants are $g_i = C'^2 V_{\text{DC}}^2 Z_i/m$ for a port with input impedance $Z_i$.

To understand the effect on the mechanics we write

$$I = \frac{1 - S_{11}}{Z_1} V_1^+ + \frac{S_{12}}{Z_1} V_2^+, \tag{S46}$$

where $V_2$ is the incident voltage wave on port 2. In analogy with Sec. IV D 3 a find

$$x = \overline{\chi}_m \left( \sqrt{\frac{g_1}{m}} v_1^+ + \sqrt{\frac{g_2}{m}} v_2^+ \right) \tag{S47}$$

We can now determine which port the mechanical oscillator thermalizes to in the strong-coupling limit that $g_1 + g_2 \gg \kappa_{\text{in}}$. In the limit of equal line impedances $g_1 = g_2$ and thermal fluctuations enter in equally from the two ports. In the more general case

$$S_{\text{xx}} = \frac{|\overline{\chi}_m|^2}{m} \left( g_1 S_{1+,1+} + g_2 S_{2+,2+} \right). \tag{S48}$$

We see that the mechanical oscillator will thermalize to a weighted sum of the temperatures from the two ports.

### *4. Dissipation and resonant transmission*

Dissipation associated with $\kappa_{\text{in}}$ can be easily incorporated by adding a third virtual port with impedance $Z_3$ given by

$$Z_3 = \frac{m\kappa_{\text{in}}}{C'^2 V_{\text{DC}}^2}. \tag{S49}$$

To understand the consequences, consider a model with one physical port and with mechanical dissipation coupled through a virtual port $v$. Imagine for simplicity that the physical port is at zero temperature. The voltage fluctuations measured at port 1 are then only those originating from the virtual port, satisfying $v_1^- = S_{13} v_3^+$, where we can read off the transmission coefficient from the two-port model. The fluctuations at port 1 then satisfy

$$S_{1-,1-} = 4 g_1 \kappa_{\text{in}} \omega^2 |\overline{\chi}_m|^2 k_B T. \tag{S50}$$

The thermo-mechanical noise transmitted on resonance is then

$$S_{1-,1-} = \frac{4 g_1 \kappa_{\text{in}}}{(g_1 + \kappa_{\text{in}})^2} k_B T. \tag{S51}$$

We see that thermo-mechanical noise is resonantly transmitted when the impedance matching condition $g_1 = \kappa_{\text{in}}$ is satisfied.

### *5. Input-output theory*

In analogy with cavity optomechanics, these findings can be neatly summarized by an input-output theory. This will give the same results as the impedance formalism, but is more convenient. The fundamental input-output relation derived from $q = CV$ and neglecting gate capacitances is

$$v_i^- = v_i^+ - i\omega\sqrt{g_i m} x. \tag{S52}$$

This must be combined with the equations of motion for $x$,

$$x = 2\sqrt{\frac{g_i}{m}} \overline{\chi}_m v_i^+, \tag{S53}$$

where as before $\overline{\chi}_m$ is the damped linewidth, and the sum over $i$ is implied by the repeated index. Scattering parameters $S_{ij} = \langle v_i / v_j \rangle$ and power spectra can be immediately derived from the above equations.

### E. Parametric gain

Mechanical parametric amplification was first studied in Ref. [58]. Later work studied gain in the presence of a cavity and generalized to non-zero detunings in Ref. [59].

Imagine the case where a voltage is applied at twice the mechanical frequency. Due to the electromechanical spring effect, this introduces a parametric shift in the mechanical frequency $\Omega_0^2 h_0 \sin(2\Omega_m t)$ where $h_0 = 2V_{2\Omega_m}/V_{\mathrm{DC}}$. According to Ref. [58] we should expect mechanical gain in a single quadrature. The equation of motion of the membrane becomes:

$$\ddot{x} + \kappa_{\mathrm{in}}\dot{x} + \Omega_m^2 x(1 + h_0 \sin(2\Omega_m t)) = F/m. \tag{S54}$$

To solve, we introduce quadrature components $x_I$ and $x_Q$,

$$x = x_I(t)\cos(\Omega_m t) + x_Q(t)\sin(\Omega_m t), \tag{S55}$$

which can be encoded by quadrature vectors $\vec{x} = (x_I, x_Q)$, with a similar decomposition for $F$. Keeping only terms varying at $\Omega_m$, the equations of motion become

$$\ddot{\vec{x}} + \kappa_{\mathrm{in}}\dot{\vec{x}} + 2\Omega_m i\boldsymbol{\sigma_y}\dot{\vec{x}} + \kappa_{\mathrm{in}}\Omega_m i\boldsymbol{\sigma}_y\vec{x} + \frac{\Omega_m^2 h_0}{2}\boldsymbol{\sigma}_x\vec{x} = \frac{1}{m}\vec{F}, \tag{S56}$$

where $\boldsymbol{\sigma}_x$ and $\boldsymbol{\sigma}_y$ are Pauli matrices in quadrature space. Changing into frequency domain, we can collect terms

$$(-\omega^2 + i\kappa_{\mathrm{in}}\omega)\vec{x} + \Omega_m(\kappa_{\mathrm{in}} + 2i\omega)i\boldsymbol{\sigma}_y\vec{x} + \frac{\Omega_m^2 h_0}{2}\boldsymbol{\sigma}_x\vec{x} = \frac{1}{m}\vec{F}, \tag{S57}$$

or explicitly as a $2x2$ matrix equation

$$\begin{pmatrix} -\omega^2 + i\kappa_{\mathrm{in}}\omega & \frac{\Omega_m^2 h_0}{2} + \Omega_m\kappa_{\mathrm{in}} + 2i\Omega_m\omega \\ \frac{\Omega_m^2 h_0}{2} - \Omega_m\kappa_{\mathrm{in}} - 2i\Omega_m\omega & -\omega^2 + i\kappa_{\mathrm{in}}\omega \end{pmatrix}\begin{pmatrix} x_I \\ x_Q \end{pmatrix} = \frac{1}{m}\begin{pmatrix} F_I \\ F_Q \end{pmatrix}. \tag{S58}$$

This matrix is easily invertible to solve for $x_I$ and $x_Q$. This gives quadrature susceptibilities

$$\begin{pmatrix} x_I \\ x_Q \end{pmatrix} = \begin{pmatrix} \chi_0 & \chi_{12} \\ \chi_{21} & \chi_0 \end{pmatrix}\begin{pmatrix} F_I/m \\ F_Q/m \end{pmatrix} \tag{S59}$$

with

$$\chi_0 = \frac{i\omega(\kappa_{\mathrm{in}} + i\omega)}{(\kappa_{\mathrm{in}} + 2i\omega)^2\Omega_m^2 - (\kappa_{\mathrm{in}} + i\omega)^2\omega^2 - h_0^2\Omega_m^4/4} \tag{S60}$$

$$\chi_{12} = \frac{-\Omega_m\kappa_{\mathrm{in}} - 2i\omega\Omega_m - \Omega_m^2 h_0/2}{(\kappa_{\mathrm{in}} + 2i\omega)^2\Omega_m^2 - (\kappa_{\mathrm{in}} + i\omega)^2\omega^2 - h_0^2\Omega_m^4/4} \tag{S61}$$

$$\chi_{21} = \frac{\Omega_m\kappa_{\mathrm{in}} + 2i\omega\Omega_m - \Omega_m^2 h_0/2}{(\kappa_{\mathrm{in}} + 2i\omega)^2\Omega_m^2 - (\kappa_{\mathrm{in}} + i\omega)^2\omega^2 - h_0^2\Omega_m^4/4} \tag{S62}$$

On resonance ($\omega = 0$) $\chi_0 = 0$, and it is small for all frequencies in the high-$Q$ limit. The gains are $G_{ij} = \chi_{ij}(h_0 \neq 0)/\chi_{ij}(h_0 = 0)$, with zero-frequency ($\omega = 0$) values

$$G_{12}^0 = G_A = \frac{\kappa_{\mathrm{in}}}{\kappa_{\mathrm{in}} - \Omega_m h_0/2}, \; G_{21}^0 = G_S = \frac{\kappa_{\mathrm{in}}}{\kappa_{\mathrm{in}} + \Omega_m h_0/2}. \tag{S63}$$

The solution for $x_{Q/I}(\omega)$ can be approximated by a Lorentzian with a height $G_{A/S}$ and a bandwidth $\kappa_{\mathrm{in}}/G_{A/S}$,

$$\begin{pmatrix} x_I \\ x_Q \end{pmatrix} \approx \frac{1}{\kappa_{\mathrm{in}}\Omega_m}\begin{pmatrix} 0 & \frac{i\kappa_{\mathrm{in}}/2}{\omega - i\kappa_{\mathrm{in}}/(2G_A)} \\ \frac{-i\kappa_{\mathrm{in}}/2}{\omega - i\kappa_{\mathrm{in}}/(2G_S)} & 0 \end{pmatrix}\begin{pmatrix} F_I/m \\ F_Q/m \end{pmatrix} = \frac{1}{m}\boldsymbol{\chi}_m\vec{F}, \tag{S64}$$

where the last equality defines the matrix susceptibility $\boldsymbol{\chi}_m$.

We can redefine the equation of motion in terms of a gain function ($\boldsymbol{G}$) and an undriven susceptibility $\boldsymbol{\chi}_m^0$:

$$\vec{x} = \frac{1}{m}\boldsymbol{G}\boldsymbol{\chi}_m^0 \vec{F} \tag{S65}$$

with

$$\boldsymbol{G} = \begin{pmatrix} \frac{\omega - \frac{i\kappa_{\rm in}}{2}}{\omega - i\kappa_{\rm in}/(2G_A)} & 0 \\ 0 & \frac{\omega - \frac{i\kappa_{\rm in}}{2}}{\omega - i\kappa_{\rm in}/(2G_S)} \end{pmatrix} \tag{S66}$$

$$\boldsymbol{\chi}_m^0 = \frac{1}{\kappa_{\rm in}\Omega_m} \begin{pmatrix} 0 & \frac{i\kappa_{\rm in}/2}{\omega - i\kappa_{\rm in}/2} \\ \frac{-i\kappa_{\rm in}/2}{\omega - i\kappa_{\rm in}/2} & 0 \end{pmatrix} \tag{S67}$$

### 1. *Quadrature input-output theory*

Since the parametric gain problem was solved in terms of quadratures, we need a quadrature input-output theory in analogy to Sec. IV D 5. From the derivative rule $\dot{x} \to \Omega_m \boldsymbol{\sigma}_y \vec{x} + \dot{\vec{x}}$, we find the relation analogous to Eq. S52,

$$\vec{v}_j^- = \vec{v}_j^+ - i\sqrt{g_j m}(\Omega_m \boldsymbol{\sigma}_y + \omega)\vec{x}. \tag{S68}$$

We now need to write the quadrature equations of motion in terms of an input wave $\vec{v}^+$, in analogy with Eq. S53. Writing $\vec{F}$ in terms of the total voltage and eliminating the out-going wave $\vec{v}^-$ using Eq. S68 gives

$$\frac{\vec{F}}{m} = 2\sqrt{\frac{g_j}{m}}\vec{v}_j^+ - ig_j(\Omega_m \boldsymbol{\sigma}_y + \omega)\vec{x}, \tag{S69}$$

where for multiple ports one must simply sum the right side over $j$. The first term on the right-hand side is the force due to the incoming wave. The second term can by identified, after substitution into Eq. S57, as introducing an effective damping at rate $g_j$. The linearized of motion can now be written down

$$\vec{x} = 2\sqrt{\frac{g_j}{m}}\overline{\boldsymbol{\chi}}_m \vec{v}^+, \tag{S70}$$

where the dressed susceptibility $\overline{\boldsymbol{\chi}}_m$ is the same as $\boldsymbol{\chi}_m$ but with an effective linewidth $\kappa_{\rm eff} = \kappa_{\rm in} + g_j$. Additional ports can be added by introducing more summands into the above equation.

These input-output relations make it straightforward to calculate scattering parameters and power spectral densities in the presence of gain. To get tidy expressions, we can neglect the $\omega$ in Eq. S68, valid when the position quadratures are slowly varying ($\omega \ll \Omega_m$), which gives the scattering formula

$$\vec{v}_j^- = (1 + \boldsymbol{\chi}_{jj}^{\rm lin})\vec{v}_j^+ + \boldsymbol{\chi}_{jk}^{\rm lin}\vec{v}_k^+ + \dots , \tag{S71}$$

where the linearized susceptibility is

$$\boldsymbol{\chi}_{jk}^{\rm lin} = -2i\sqrt{g_j g_k}\Omega_m \boldsymbol{\sigma}_y \boldsymbol{\chi}_m = \begin{pmatrix} \frac{i\sqrt{g_j g_k}}{\omega - i\kappa_{\rm eff}/(2G_S)} & 0 \\ 0 & \frac{i\sqrt{g_j g_k}}{\omega - i\kappa_{\rm eff}/(2G_A)} \end{pmatrix} \tag{S72}$$

and the ... denote analogous terms for more ports. We finally see that that the output modes consists of a prompt-reflected input mode, plus each mode squeezed in phase and amplified out of phase. This expression is reminiscent of Eq. S44. In fact, when there is no gain ($h_0 = 0$, $G_A = G_S = 1$), we have $\boldsymbol{\chi}_m = \frac{-1}{\kappa_{\rm in}\Omega_m}\frac{\kappa_{\rm in}/2}{\omega - i\kappa_{\rm in}/2}\boldsymbol{\sigma}_y$, and we arrive at a linearized version of Eq. S44.

Power spectra are also straightforward at the level of Eq. S71 because all matrices are diagonal; there are no cross-correlations between quadratures.

### 2. *Position inference*

From the previous section, in particular Eq. S71, it's trivial to write the outgoing power spectral density $S_{--}$ in terms of the incoming ones $S_{++}$. It's less trivial to relate $S_{--}$ to the position spectral density $S_{xx}$. This is trickier because $\vec{v}_j^+$ and $\vec{x}$ are correlated. We need to work with a power spectral matrix $BW\vec{v}_j^- \otimes \vec{v}_j^{*-}$, where $BW$ is the measurement bandwidth and $\otimes$ is the outer product. Assuming the input field is in a thermal state, $\vec{v}_i^+ \otimes \vec{v}_j^{*+} = k_B T \delta_{ij}$, we find the power spectral matrix

$$\boldsymbol{S}_{--} = (1 + 2\mathrm{Re}[\boldsymbol{\chi}_{11}^{\mathrm{lin}}])k_B T + gm\Omega_m^2 \boldsymbol{S}_{\mathrm{xx}}, \tag{S73}$$

where $\mathrm{Re}[x]$ denotes the real part of $x$ and we have labeled the measurement port as $j = 1$. As a check, one can verify that without gain and with only one input field, the above expression is equal to $k_B T$, which is expected because our quadrature definition gives $\langle x^2 \rangle = \langle x_I^2 \rangle/2 + \langle x_Q^2 \rangle/2$.

#### a. *Undriven Position Fluctuations*

We can now combine equations (S65) and (S70) to write the position fluctuations in terms of an undriven susceptibility and the incoming scattering waves at port i:

$$\boldsymbol{S}_{xx,i} = 4\frac{g_i}{m}|\boldsymbol{G}|^2|\overline{\boldsymbol{\chi}}_m^0|^2 \boldsymbol{S}_{i+i+}. \tag{S74}$$

The total undriven position fluctuations ($\boldsymbol{S}_{xx} = |\boldsymbol{G}|^2 \boldsymbol{S}_{xx}^0$) is the sum of the fluctuation contributions from each port i:

$$\boldsymbol{S}_{xx}^0 = \frac{4}{m}|\overline{\boldsymbol{\chi}}_m^0|^2 \sum_i g_i \boldsymbol{S}_{i+i+} = \frac{1}{m\Omega_m^2}\frac{\kappa}{\omega^2 + (\kappa/2)^2}\sum_i \frac{g_i}{\kappa}\boldsymbol{S}_{i+i+}. \tag{S75}$$

We can define the undriven bath temperature ($T_m$) as the average of the incoming radiation, weighted by the coupling:

$$k_B T_m = \sum_i \frac{g_i}{\kappa}\boldsymbol{S}_{i+i+}. \tag{S76}$$

On resonance the expression for the bath temperature reduces to $m\Omega_m^2 \boldsymbol{S}_{xx} = 4k_B T_m$. In the high gain limit, the outgoing power spectral density can be approximated from the position fluctuations:

$$\boldsymbol{S}_{--} = gm\Omega_m^2 |\boldsymbol{G}|^2 \boldsymbol{S}_{xx}^0. \tag{S77}$$

#### b. *Area analysis*

In the experiment, we can estimate the mechanical temperature by analyzing the area of Lorentzians in power spectral density traces. A handy relation is

$$\int \frac{1}{(2\pi f)^2 + (\frac{\kappa}{2G})^2} df = \frac{G}{\kappa}. \tag{S78}$$

The area associated with the Lorentzian parts of Eq. S73 evaluates to

$$A = g\left(m\Omega_m^2 \langle x_I^2 \rangle - k_B T\right). \tag{S79}$$

In thermal equilibrium we get $A = 0$, as required for equilibrium white noise.

Imagine a situation where the input mode has a known temperature $T$, but the mechanics is coupled to additional ports that, in the absence of gain, would set it to some temperature $T_m$. $T_m$ can be understood as the temperature of the mechanical bath. Using Eq. S70 and carrying out the frequency integral for the amplified quadrature gives the area

$$A = gk_B(G_A T_m - T). \tag{S80}$$

In our experiment we measure the output mode $v_o$ from a coupler, which can be accounted for with the additional input-output relation

$$\vec{v}_o = \sqrt{\eta}\vec{v}^- + \vec{v}_{\rm add}, \tag{S81}$$

where $v_{\rm add}$ accounts both for added thermal noise due to loss the added noise of the chain. Here $\eta$ includes both the directional coupler and system losses between the sample and the measurement device. The output area $A_o$ is a factor of $\eta$ smaller than the input area $A$, so we have

$$\frac{A_o}{k_B g} = \eta G_{\rm A} T_m - \eta T. \tag{S82}$$

For simplicity, we can redefine the area as $A_{\rm eq} = A_o/(k_B g)$ and gain as $G_{\rm eq} = \eta G_A$. In addition, we need to relate the apparent gain measured in the experiment to $G_A$. The apparent gain is measured using the increase in the height of a pilot tone, as shown in the following section.

### *3. Signal recovery and apparent gain*

Imagine there is one physical port with coupling $g_1$ and a dissipation port with coupling $\kappa_{\rm in}$. For the amplified quadrature, the output noise on resonance is

$$S_{\rm mm} = \eta\left(1 - G_A\frac{2g_1}{\kappa_{\rm in}+g_1}\right)^2 S_{++} + \eta\left(G_A\frac{2\sqrt{\kappa_{\rm in}g_1}}{\kappa_{\rm in}+g_1}\right)^2 S_{00} + S_{\rm add} \tag{S83}$$

When measuring, we referred to an apparent gain $G^0_{\rm app} = \sqrt{\eta}|1 - 2G_A\frac{g_1}{\kappa_{\rm in}+g_1}|$. Inverting this expression gives $G_A$ in terms of the apparent gain,

$$G_A = \frac{\kappa_{\rm in}+g_1}{2g_1}\left(\frac{G_{\rm app}}{\sqrt{\eta}}+1\right), \tag{S84}$$

which should be used in the area analysis discussed in Sec. IV E 2 b.

The input-referred noise of the amplified quadrature is

$$S_{++} + \frac{\kappa_{\rm in}g_1}{\omega^2 + (g_1 - \kappa/(2G_A))^2}S_{00} + \frac{1}{G^2_{\rm app}}S_{\rm add}, \tag{S85}$$

where we have introduced the frequency-dependent apparent gain $G^2_{\rm app}(\omega) = |1+\chi^{\rm lin}_m|^2$, which satisfies $G_{\rm app}(0) = G^0_{\rm app}$. The second term in Eq. S85 represents the unavoidable addition of noise due to mechanical loss, and the third term is the noise added by the subsequent components, which is suppressed by gain.

For a 2-port device, i.e., a device with two physical ports and a virtual one, an analogous derivation can be done. Consider we add an incoming wave $\vec{v}_1^{*+}$ to port 1 while measuring the outgoing wave from port 2 and that the only incoming radiation at port 2 comes from its thermal fluctuations. For the amplified quadrature, the output noise on resonance is

$$S_{\rm mm} = \eta\left(1 - G_A\frac{2g}{\kappa_{\rm eff}}\right)^2 S_{2+2+} + \eta\left(G_A\frac{2g}{\kappa_{\rm eff}}\right)^2 S_{1+1+} + \eta\left(G_A\frac{2\sqrt{\kappa_{\rm in}g}}{\kappa_{\rm eff}}\right)^2 S_{00} + S_{\rm add}. \tag{S86}$$

where $\kappa_{\rm eff} = \kappa_{\rm in} + 2g$. We can once again relate the apparent gain to $G_A$

$$G_A = \frac{\kappa_{\rm eff}}{2g}\frac{G_{\rm app}}{\sqrt{\eta}}. \tag{S87}$$

## F. Converting 2-port measurement into 1-port measurement

A two-port measurement is limited by the room-temperature noise contribution of multiple ports. We would like to convert to a one-port measurement in order to minimize the noise added by ports. Naively, one could take this measurement as shown in Fig. S4(a), using a power splitter to add the reflected and transmitted portions of the signal

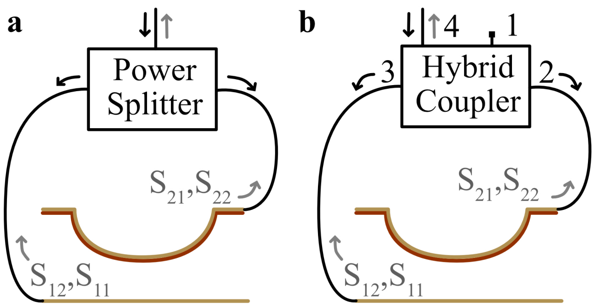


Figure S4. Two possible configurations for a one-port measurement. (a) Using a power splitter to add reflected and transmitted components. (b) Using a hybrid coupler to subtract reflected and transmitted components.

together. However, returning to (S43) and (S44) shows that when $g_1 = g_2$, $S_{21} + S_{11} = 1$. No information is gained from this measurement.

Another possible approach, as shown in Fig. S4(b), is to use a hybrid coupler, which adds a 180° phase shift to one port, in place of a power splitter. The scattering matrix of a hybrid coupler is:

$$[S] = \frac{-i}{\sqrt{2}} \begin{bmatrix} 0 & 1 & 1 & 0 \\ 1 & 0 & 0 & -1 \\ 1 & 0 & 0 & 1 \\ 0 & -1 & 1 & 0 \end{bmatrix}. \tag{S88}$$

A signal $a$ incident on port 4 of the hybrid coupler (the $\Delta$ port) will generate a signal of $-ia/\sqrt{2}$ out of port 3 and a signal of $ia/\sqrt{2}$ out of port 2, both of which will interact with the sample. We can assume reciprocity, $S_{21} = S_{12}$, and symmetry, $S_{11} = S_{22}$, which gives a signal of

$$\frac{ia}{\sqrt{2}}(S_{21} - S_{11}) \tag{S89}$$

incident on port 3. Likewise, port 2 receives a signal of

$$\frac{ia}{\sqrt{2}}(S_{11} - S_{21}). \tag{S90}$$

The hybrid coupler again modifies the signal from ports 3 and 2 by $-i/\sqrt{2}$ and $i/\sqrt{2}$, respectively, and combines them, returning a signal of

$$a(S_{21} - S_{11}). \tag{S91}$$

Returning again to (S43) and (S44), we evaluate the ratio of the returned signal to the original signal for $g_1 = g_2$:

$$S_{out} = (1 - 4i\omega g\bar{\chi}_m), \tag{S92}$$

giving us a device which is effectively converted to a one-port configuration.

### 1. *Conservation of energy in converted measurement*

Equation (S92) can be evaluated on resonance to:

$$S_{out} = 1 - \frac{4i\omega g}{i(\kappa_{\text{in}} + 2g)\omega} \tag{S93}$$

for $\kappa = \kappa_{\text{in}} + 2g$ according to (S45). In the case of zero loss ($\kappa_{\text{in}} = 0$) this works out to

$$S_{out} = 1 - \frac{4g}{2g} = -1 \tag{S94}$$

which corresponds to a sign change in voltage but no power loss. This is the same as (S44) for $g \to 2g$.

### G. Added noise temperature

We have developed a protocol to determine the added noise temperature of the CEM amplifier based on a two-point temperature calibration. The noise temperature for individual voltage trace ($V_-$) is calculated as described in IV E 2 b with $G_{\text{app}}$

$$G_{\text{app}} = \frac{V_-}{P_t/ATT}, \tag{S95}$$

where the attenuation ($ATT$) is the ratio of measured voltage fluctuations due to a probe tone and its amplitude ($P_t$). The input referred noise of the membrane amplifier $T_{\text{ref}}(G_{\text{m}})$ is calculated by $T_m/G_{\text{eq}}$ and measured for a reference resistor at RT (295 K) and LN (70 K) temperature. The intercept value of $T_{\text{ref}}(G_A)$ gives the added noise temperature ($T_{add}$) of the membrane amplifier.

### H. Cooperativity comparisons

To better understand the criteria for achieving large cavity-free cooperativity $\mathscr{C} > 1$, we have estimated what $\mathscr{C}$ could be achieved in various device geometries [Table SII]. We used the formula $\mathscr{C} = \frac{C'(x)^2 V_{DC}^2 Z_0}{m\kappa_{\text{in}}}$ of capacitively coupled mechanical resonators in the literature. We use the reported numbers for plate spacing, area, resonator dimensions and linewidth and voltage where provided. In cases where multiple resonators are studied, we compute a cooperativity typical of the regime studied.

| Reference | Projected $\mathscr{C}$ at 2 V | Projected $\mathscr{C}$ at max. voltage | Cavity-free | Voltage biased |
|---|---|---|---|---|
| [32] | $6 \times 10^{-4}$ | $2 \times 10^{-2}$ | y | y |
| [34] | $1.5 \times 10^{-4}$ | $5.1 \times 10^{-2}$ | y | y |
| [33] | $8.8 \times 10^{-7}$ | $1.1 \times 10^{-3}$ | y | y |
| [25] | $1.2 \times 10^{-5}$ | $6.5 \times 10^{-4}$ | n | y |
| [53] | $5.6 \times 10^{-4}$ | $8.9 \times 10^{-3}$ | n | y |
| [55] | 0.15 | 3.6 | n | y |
| [54] | 78 | NA | n | n |

Table SII. Projected $\mathscr{C}$ for various examples in the literature at a bias of 2 V, and at the maximum voltage studied where applicable. While no other cavity-free devices have previously reached $\mathscr{C} > 1$, some cavity-coupled devices capable of near ground-state sideband cooling are likely also capable of reaching $\mathscr{C} > 1$ without a cavity [54, 55]. Note that for Ref. [33] we project cooperativities for a silicon nitride-graphene membrane with quarter-segment electrodes, using a max voltage of 70 V, and optimistically fundamental mode quality $Q = 5 \times 10^4$. For Ref. [34] we assume that the graphene is a single layer and select the lowest mechanical decay rate out of the modes studied. For Ref. [53] Q are measured at 0V bias voltage. For Ref. [55] thickness of the aluminum drum is estimated to be 100 nm, based on a similar device geometry studied in Ref. [8]. The density of graphene is taken to be $7.4 \times 10^{-7}$ kg/m$^2$ from Ref. [60].

It is important to emphasize that no previous work has actually observed $\mathscr{C} > 1$. Indeed, common device geometries have $\mathscr{C}$ in the range $10^{-2} - 10^{-7}$ [25, 32–34, 53]. Cavity-coupled devices that are known to exhibit near ground-state sideband cooling are also projected to be capable for reaching cavity-free strong coupling $\mathscr{C} > 1$ [54, 55]. Although the requirements for ground-state cooling and cavity-free strong coupling are not identical, they both require large capacitive gradients $C'$ and small motional mass $m$.
